# Supplementary material for: Procedural Content Generation using Neuroevolution and Novelty Search for Diverse Video Game Levels
Source: arXiv:2204.06934 source file (2022-04-14)
Supplement: Supplementary file 1 [file 1_files_appendix_boiler.tex]

\usepackage{float}                  % Allows 'Here and Only Here' [H] for Floats
\usepackage{url}                    % \url{} command
\usepackage{graphicx}               % \includegraphics
\usepackage{amsmath}
\usepackage{amsthm}
\usepackage{booktabs}
\usepackage{multirow}
\usepackage{tikz}
\usetikzlibrary{positioning}
\usetikzlibrary{fit,shapes}
\usetikzlibrary{calc}
\usetikzlibrary{matrix, positioning,fit,shapes,calc}
% \usepackage[all]{nowidow}
% \setnoclub[2]
% \setnowidow[2]
\graphicspath{{../../../src/},{../../../src/}}
\usepackage{algorithm}
\usepackage{algpseudocode}

\makeatletter
\newcounter{phase}[algorithm]
\newlength{\phaserulewidth}
\newcommand{\setphaserulewidth}{\setlength{\phaserulewidth}}

\makeatother

\setphaserulewidth{.7pt}

\usepackage{subcaption}
\usepackage{adjustbox}
\usepackage[english]{babel} 
% Referencing 
% Provides \Vref and \vref to indicate where a reference is.
\usepackage{varioref} 
% Hyperlinks references
% Provides \Cref, \cref, \Vref, \vref to include the type of reference: fig/eqn/tbl
\usepackage[nameinlink]{cleveref}
% Setup Hyperref
\hypersetup{
  colorlinks   = true,              %Colours links instead of ugly boxes
  urlcolor     = black,              %Colour for external hyperlinks
  linkcolor    = black,              %Colour of internal links
  citecolor    = black                %Colour of citations
}
% Names for Clever Ref
\crefname{table}{table}{tables}
\Crefname{table}{Table}{Tables}
\crefname{figure}{figure}{figures}
\Crefname{figure}{Figure}{Figures}
\crefname{equation}{equation}{equations}
\Crefname{equation}{Equation}{Equations}
\addto\extrasenglish{  
    
}
\addto\extrasenglish{  
    
}
\addto\extrasenglish{  
    
}
\addto\extrasenglish{  
    
}

% \addto\extrasenglish{  
%   \def\figureautorefname{Fig.}  
% }

% \addto\extrasenglish{  
%   \def\figurename{Figure}  
% }
\addto\extrasenglish{  
    
}
\addto\extrasenglish{  
    
}

\addto\extrasenglish{  
    
}
\algnewcommand{\LineComment}[1]{\State \(\triangleright\) #1}

\algnewcommand{\LeftComment}[1]{\(\triangleright\) #1}
\algnewcommand{\TestLineComment}[1]{// #1}

% ~\ref*{#1}
\newcommand{\refappendix}[1]{\hyperref[#1]{Appendix}}

\makeatletter
\newcommand*{\centerfloat}{%
  \parindent \z@
  \leftskip \z@ \@plus 1fil \@minus \textwidth
  \rightskip\leftskip
  \parfillskip \z@skip}
\makeatother

\makeatletter
\newcommand\Autoref[1]{\@first@ref#1,@}
\def\@throw@dot#1.#2@{#1}% discard everything after the dot
\def\@set@refname#1{%    % set \@refname to autoefname+s using \getrefbykeydefault
    \edef\@tmp{\getrefbykeydefault{#1}{anchor}{}}%
    \xdef\@tmp{\expandafter\@throw@dot\@tmp.@}%
    \ltx@IfUndefined{\@tmp autorefnameplural}%
         {\def\@refname{\@nameuse{\@tmp autorefname}s}}%
         {\def\@refname{\@nameuse{\@tmp autorefnameplural}}}%
}
\def\@first@ref#1,#2{%
  \ifx#2@\autoref{#1}\let\@nextref\@gobble% only one ref, revert to normal \autoref
  \else%
    \@set@refname{#1}%  set \@refname to autoref name
    \@refname~\ref{#1}% add autoefname and first reference
    \let\@nextref\@next@ref% push processing to \@next@ref
  \fi%
  \@nextref#2%
}
\def\@next@ref#1,#2{%
   \ifx#2@ and~\ref{#1}\let\@nextref\@gobble% at end: print and+\ref and stop
   \else, \ref{#1}% print  ,+\ref and continue
   \fi%
   \@nextref#2%
}

\makeatother

\fboxsep=-0.2mm%padding thickness
% \fboxrule=0.1pt%border thickness
\makeatletter
\renewcommand*{\NAT@spacechar}{~}
\makeatother
